# Supplementary material for: Definability of linear equation systems over groups and rings
Source: arXiv:1204.3022 source file (2013-11-11)
Supplement: Supplementary file 1 [file further-background.tex]

We provide further background reading for the topics considered in this paper.

% -----------------------------------------------------------------------------
% Lindstrom quantifiers and extensions
% -----------------------------------------------------------------------------
\subsection{Lindstr\"om quantifiers and extensions}

Generalised quantifiers in the sense of Lindstr\"om~\cite{lindstroem66genQuantifiers} have been studied as a way to increase the expressiveness of a logic by a prescribed query. Let $\sigma = (R_1, \dots, R_l)$ be a vocabulary where each relation $R_i$ has arity $n_i$. Consider a class $\structClass K$ of $\sigma$-structures that is closed under isomorphism; that is, for $\sigma$-structures $\struct A$ and $\struct B$, if $\struct A \in \structClass K$ and $\struct A \isom \struct B$, then $\struct B \in \structClass K$. With $\structClass K$ we associate a \emph{Lindstr\"om quantifier} $\lindstrom K$ whose \emph{type} is the tuple $(n_1, \ldots, n_l)$. The \emph{arity} of the quantifier $\lindstrom K$ is the value of $\max\{ n_1, \dots, n_l\}$. For a logic $\logic L$, define the extension $\logic{L}(\lindstrom K)$ by closing the set of formulae of $\logic L$ by introducing the following formula-formation rule:

\begin{quote}
if $\phi_1, \dots, \phi_l$ are formulae of $\logic{L}(\lindstrom K)$, $\tup x_1, \dots, \tup x_l$ tuples of variables where $\tup x_i$ has length $n_i$, then the expression $\lindstrom{K} \tup x_1 \dots \tup x_l \qsep (\phi_1, \dots, \phi_l)$ is a formula of $\logic{L}(\lindstrom K)$ with all occurrences of $\tup x_i$ in $\phi_i$ bound.
\end{quote}

\noindent The semantics of the Lindstr\"om quantifier $\lindstrom K$ is defined such that
\begin{quote}
	$\struct A \models \lindstrom{K} \tup x_1 \dots \tup x_l \qsep (\phi_1, \dots, \phi_l)$ if and only if $(\univ A; \phi_1(\tup x_1)^\struct{A}, \dots, \phi_l(\tup x_l)^\struct{A}) \in \structClass K$,
\end{quote}

\noindent where $(\univ A; \phi_1(\tup x_1)^\struct{A}, \dots, \phi_l(\tup x_l)^\struct{A})$ is interpreted as a $\sigma$-structure. 

Similarly we can consider the extension of a logic $\logic L$ by a collection $\mathbf Q$ of Lindstr\"om quantifiers. The logic $\logic L(\mathbf Q)$ is defined by adding a rule for constructing formulae with the quantifier $Q$, for each $Q \in \mathbf Q$, to the list of formula-formation rules for $\logic L$. The semantics is defined by considering the semantics for each quantifier $Q \in \mathbf Q$, as above.

Often we consider families of quantifiers generated under some uniformity condition. Here we focus on the following notion of uniformity, due to Dawar~\cite{dawar95generalized}. Let $\structClass K$ be a class of structures over vocabulary $\sigma = (R_1, \dots, R_l)$. For each $m \in \N$, let $\sigma_m$ be the vocabulary $(R_{m,1}, \dots, R_{m,l})$ where the arity of $R_{m,i}$ is $m \cdot n_i$. Let $\structClass K_m$ be the class of $\sigma_m$-structures defined by
\[
	\structClass K_m \defeq \{ (A, S_1, \dots, S_l) \sep (A^m, S_1, \dots, S_l) \in \structClass K \},
\]

\noindent 
where $(A^m; S_1, \dots, S_l)$ is seen as a $\sigma$-structure with universe $A^m$. If $Q_m$ is the Lindstr\"om quantifier associated with $\structClass K_m$ then we say that the sequence $\uniformLindstrom K \defeq \{ Q_m \sep m \in \N \}$ is \emph{uniformly generated by $\structClass K$}. 

\begin{definition}[Uniform sequences of quantifiers]
A countable collection $\mathbf Q$ of Lindstr\"om quantifiers is a \emph{uniform sequence} if there is a class of structures $\structClass K$ such that $\mathbf Q = \uniformLindstrom K$.
\defnend
\end{definition}

% -----------------------------------------------------------------------------
%
% Linear Algebra
%
% -----------------------------------------------------------------------------
\subsection{Linear algebra}
\label{sec_linear-algebra}

A matrix is usually regarded as a rectangular grid of elements, with rows and columns given in a particular order. However, most natural matrix properties are well-defined if we consider a more generic notion of a matrix, where the rows and columns are indexed by arbitrary unordered sets. In this section we introduce \emph{unordered matrices} of this kind and review some basic linear algebra. 

% 
% Elementary linear algebra
% 
\subsubsection{Matrices and linear maps}

Let $R$ be a commutative ring. An \emph{$m \times n$ matrix over $R$} is a rectangular array of scalars from $R$, consisting of $m$ rows and $n$ columns. We write $m \times n$ for the \emph{dimension} of $A$. An $m \times n$ matrix is said to be \emph{square} (of order $n$) if $m = n$. We write $A = (a_{ij})_{1 \leq i \leq m, 1 \leq j \leq n}$ (or $A = (a_{ij})$ for short when the dimension of $A$ is clear from the context) to denote the matrix
\[
	A = 
	\begin{pmatrix}
		a_{11} 	& 	\cdots 	& 	a_{1n} 	\\
		\vdots	&	\ddots	&	\vdots	\\
		a_{m1} 	& 	\cdots 	& 	a_{mn} 	\\
	\end{pmatrix}.
\]

\noindent
When $R = F$ is a field, a matrix over $F$ can alternatively be seen to represent a linear map between two finite-dimensional vector spaces, given a basis for each vector space. To see this, we first recall some basic definitions from elementary linear algebra. Let $U$ be an $n$-dimensional vector space over a field $F$ and let $B = \{u_1, \dots, u_n\}$ be an \emph{ordered} basis for $U$, where $u_1 < u_2 < \dots < u_n$. With respect to this basis, we can represent each element $x$ of $U$ as an $n$-tuple $[x]_{B} \defeq (a_1, \dots, a_n) \in F^n$, where $x = a_1 u_1 + \cdots + a_n u_n$ is the unique expression of $x$ in terms of the basis elements of $B$. The scalars $a_i$ are called the \emph{coordinates} of $x$ with respect to the basis $B$ and $[x]_{B}$ is the unique \emph{$B$-coordinate representation of $x$}. It is not hard to see that the map $U \rightarrow F^n$, $x \mapsto [x]_{B}$ is an isomorphism of vector spaces. 

Now consider an $n$-dimensional vector space $U$ and an $m$-dimensional vector space $V$ over the same scalar field $F$. Let $B_U = \{u_1, \dots, u_n\}$ be a basis for $U$ and let $B_V = \{v_1, \dots, v_m\}$ be a basis for $V$. If $T: U \rightarrow V$ is a linear map then we construct an $m \times n$ matrix $A$ as follows. For each $u_i \in B_U$, let $[T(u_i)]_{B_V} = a_{1i} v_1 + \cdots + a_{mi} v_m$ and let $A \defeq (a_{ij})$ denote the matrix obtained by gathering all the coefficients $a_{ij}$. We call $A$ the \emph{matrix representing $T$ with respect to bases $B_U$ and $B_V$}. It can be seen that for any $x \in U$, $[T(x)]_{B_V} = A ([x]_{B_U})$. Observe that here the ordering of each basis is important. That is, changing the ordering of a given basis amounts to permuting the rows and columns of the associated matrix representation.

By this discussion, every linear map can be represented by a matrix, given suitable bases for both its domain and co-domain. Moreover, every matrix can be seen as a representation of some linear map. More specifically, let $A$ be an $m \times n$ matrix over a field $F$. Then $A$ is the matrix of the linear map $T: F^n \rightarrow F^m$, defined for all $x \in F^n$ by $T(x) \defeq A x$, where $x$ is seen as a column vector of length $n$ over $F$. The \emph{image} of $A$ is the image $\{ Ax \sep x \in F^n \} \subseteq F^m$ of the associated linear map and the \emph{null-space} (or \emph{kernel}) of $A$ is $\{ x \in F^n \sep Ax = 0 \} \subseteq F^n$. The \emph{rank} of the matrix $A$ is the dimension of its image and the \emph{nullity} of $A$ is the dimension of its null-space. A fundamental result of elementary linear algebra is the relation
\begin{quote}
	$n$ = dimension of the image of $A$ + dimension of the null-space of $A$,
\end{quote}

\noindent
often referred to as the \emph{rank-nullity theorem}.

% 
% Unordered matrices
% 
\subsubsection{Matrices and vectors indexed by arbitrary sets}

Rank and nullity are two examples of matrix properties that are in fact properties of the underlying linear map that the matrix represents. The same holds for many common matrix properties that we focus on in linear algebra; for example determinant and singularity. It follows from the above discussion that such natural matrix properties are invariant under permutation of the rows and columns of the matrix, since the associated linear map is invariant under a permutation of the chosen vector space bases. With this in mind, it is natural to consider a more general notion of a matrix, where the rows and columns are indexed by arbitrary \emph{unordered} sets. 

\makebreak

\noindent
Let $R$ be a commutative ring and let $I$, $J$ be finite, non-empty sets. An \emph{$I \times J$ matrix} $A$ over $R$ is a function $A: I \times J \rightarrow R$, where the rows of $A$ are indexed by $I$ and the columns of $A$ are indexed by $J$. We write $A = (a_{ij})$ to denote that $A(i,j) = a_{ij}$ for all $i \in I $ and $j \in J$. If $I = J$ then $A$ is called a \emph{square matrix}. We often identify relations $A \subseteq I \times J$ with the $(0,1)$-matrix defined by the characteristic function of $A$; in this case the actual co-domain is usually clear from the context. If $A$ is an $I \times J$ matrix then the \emph{dimension} of $A$ is $\card{I} \times \card{J}$. 

By taking $I = [m]$ and $J = [n]$ we get the more familiar notion of an ordered $m \times n$ matrix; i.e. a rectangular array of elements consisting of $m$ rows and $n$ columns. Most natural matrix properties, such as determinant and rank over a field, apply directly to matrices indexed by arbitrary unordered sets sets. 

\noindent
We also consider vectors indexed by arbitrary sets. That is, if $I$ is finite and non-empty, then a \emph{vector indexed by $I$} over a commutative ring $R$ is a function $b: I \rightarrow R$. 

\makebreak

\noindent
Addition and multiplication of unordered matrices is defined in exactly the same way as for ordered matrices, except that we now have to ensure that the index sets of the two matrices, and not just their dimension, are matching. That is, if $A$ and $B$ are two $I \times J$ matrices then their sum $A + B$ is the $I \times J$ matrix defined for all $i \in I$ and $j \in J$ by $(A+B)(i,j) \defeq A(i,j) + B(i,j)$. Similarly, if $A$ is an $I \times K$ matrix and $B$ is a $K \times J$ matrix, where all index sets are finite and non-empty, then the product of $A$ and $B$ is the $I \times J$ matrix $AB$ defined for all $i \in I$ and $j \in J$ by $(AB)(i,j) \defeq \sum_{k \in K}A(i,k)B(k,j)$.

%For a two-sorted $\tau_M$-structure $\mfA = ( (A,R), M , +, \cdot)$ such that $A,R$ are disjoint sets and $(R,+,\cdot)$ is a commutative ring with identity, let  $I^\mfA = \lbrace a \in A : \exists b \in A, r \in R : (a,b,r) \in M \rbrace$ and $J^\mfA = \lbrace b \in A : \exists a \in A, r \in R: (a,b,r) \in M \rbrace$. Then the structure $\mfA$ encodes the $I^\mfA \times J^\mfA$ matrix $M^\mfA$ over $R^\mfA=(R,+,\cdot)$ defined as $M^\mfA(a,b) := \sum_{(a,b,r) \in R} r$ (where the empty sum is considered to be $0 \in R$). A structure $\mfA$ encodes a square matrix if $I^\mfA = J^\mfA$. Let $N$ be a further ternary relation symbol of mixed arity $(2,1)$ and $\tau_{M,N} := \tau_M \cup \lbrace N \rbrace$. Besides the matrix $M^\mfA$, a $\tau_{M,N}$-structure $\mfA$ additionally encodes an $K^\mfA \times L^\mfA$ matrix $N^\mfA$ in totally analogous fashion. Similarly, let $b$ be a binary relation symbol of mixed arity $(1,1)$ and $\tau_{M,b}:= \tau_M \cup \lbrace b \rbrace$, then a $\tau_{M,b}$-structure $\mfA$ additionally encodes a column vector $b^\mfA$. We understand $\tau_{M,b}$-structures $\mfA$ as encoding linear equation systems $\mcS^\mfA$, where $M^\mfA$ is the coefficient matrix and $b^\mfA$ its solution vector.

% --- Systems of equations over groups and rings ------------------------------
\subsubsection{Systems of linear equations over groups and rings}

%\footnote{We can define a system of equations over any finite group $G$, except that when $G$ is non-Abelian then $G$ is not a $\Z$-module. In that case, an equation $a_1 \cdot x_1 + a_2 \cdot x_2 + \cdots + a_m \cdot x_m = g$ has the restriction that $a_i \in \{-1,0,1\}$ for all $i$, where $a_i = 0$ indicates that $x_i$ does not appear in the equation, $a_i = 1$ indicates that $x_i$ does appear in the equation and $a_i = -1$ indicates that the inverse of $x_i$ appears in the equation. For an Abelian group $G$, there is an easy first-order reduction from a system of equations $A \vec x = \vec b$ over $G$ with $\Z$-coefficients to an equivalent system $A' \vec x = \vec b'$ over $G$ where all coefficients are in $\{-1,0,1\}$.}

Let $G$ be a finite Abelian group, written additively with identity $e$. An equation over $G$ is an expression of the form
\begin{equation}
\label{eqn_equation-over-abelian-group}
	\sum_{j \in J} v_j = g
\end{equation}

\noindent 
where $g \in G$, $J$ is finite and non-empty, and each $v_j$ is either a variable $x_j$ or an inverted variable $(-x_j)$. The expression (\ref{eqn_equation-over-abelian-group}) can be \emph{satisfied} if there is an assignment of values from $G$ to the variables so that the equality holds. A system of equations over $G$ is a collection $S$ of equations of this kind. We can assume, without loss of generality, that such a system contains only variables and no inverted variables. Otherwise, we can consider the system of equations obtained from $S$ by replacing every occurence of an inverted variable $(-x_j)$ with a new variable $x_j^{\text{neg}}$ and including an additional equation $x_j + x_j^{\text{neg}} = e$. With this assumption, we can write a system of equations over $G$ as a matrix equation $A \vec x = \vec b$, where $A \in \lbrace 0,1 \rbrace^{I \times J}$, $\vec b \in \struct{G}^I$, $\vec x$ is a $J$-vector of variables taking values in $G$ and $I,J$ are finite non-empty sets. A system $A \vec x = \vec b$ is said to be \emph{solvable} if there is an assignment of values which simultaneously satisfies each equation; that is, if there is a vector $\vec c \in \struct{G}^J$ such that $A \vec c = \vec b$, where matrix multiplication takes place in $G$ as a $\Z$-module. 

More often, we consider equations where the variables are allowed to take values in a commutative ring rather than simply a group. Let $R$ be a commutative ring and write $+$ and $\cdot$ for addition and multiplication in $R$, respectively. A linear equation over $R$ is an expression of the form
\[
	\sum_{j \in J} a_j x_j = b
\]

\noindent 
where $b \in R$ is a constant, each $x_j$ is a variable and each scalar coefficient $a_j$ is an element of $R$. A system of linear equations over $R$ (or \emph{linear system}, for short) is a collection of such expressions; the system is said to be solvable if there is an assignment of the variables to elements in $R$ that simultaneously satisfies each equation. A linear system over a ring can be described succinctly as a matrix equation $A \vec x = \vec b$, where $A \in \struct{R}^{I \times J}$, $\vec b \in \struct{R}^I$, $\vec x$ is a $J$-vector of variables taking values in $R$ and $I,J$ are finite non-empty sets.
