# Supplementary material for: Definability of linear equation systems over groups and rings
Source: arXiv:1204.3022 source file (2013-11-11)
Supplement: Supplementary file 2 [file les-different-domains-proofs.tex]

%--------------------------------------------------------------------------
% From ordered non-commutative to cyclic groups
%--------------------------------------------------------------------------

In the following, we give a fixed-point Turing-reduction from solvability over arbitrary ordered finite rings to solvability over cyclic groups of prime-power order.

%\theoremreductionordgenringslcon
\begin{theorem}
$\SolveGeneralOrdRing \fpleqTur \LCON$. 
\end{theorem}

\begin{proof} 
The proof follows the same lines as the proof of
Theorem~\ref{theorem_reduction-ordings-lcon}.
Again, we use the linear order to identify a (minimal) set $\{
g_1, \dots, g_k \} \subseteq R$ which generates the additive
group $(R,+)$ of~$R$ such that $\ord{(g_1)} \divides \ord{(g_2)} \divides
\cdots \divides \ord{(g_k)} := m$ and $(R,+) \cong \langle g_1 \rangle
\oplus
\langle g_2\rangle \oplus \cdots
\oplus \langle g_k\rangle$. We do not require the ring $R$ to contain
a multiplicative identity, so we use the subgroup generated by $g_k$ to
interpret a cyclic group $\Zm{m}$. Accordingly, every element of
$R$ can be represented by a $k$-tuple of elements in $\langle g_k
\rangle =
\Zm{m}$ (where we make use of the fact that $\langle g_i \rangle$ is
isomorphic to a subgroup of $\langle g_k \rangle$ since $\ord{(g_i)}
\divides
\ord{(g_k)}$).

In order to translate the linear system $(A, \fvec b)$ over $R$ into an
equivalent system $(A^\star, \fvec b^\star)$ over $\Zm{m}$ we proceed
as before: firstly, we substitute every variable $x$ ranging over $R$ by
a tuple $(x_1,x_2, \dots, x_k)$ of variables ranging over the appropriate
subgropups of $\Zm{m}$. Secondly, we rewrite all linear terms that occur in
the
equation system with respect to this representation of $(R,+)$. In
contrast to the proof of Theorem~\ref{theorem_reduction-ordings-lcon} we
have to
distinguish between terms $rx=(r_1,\dots,r_k)(x_1,\dots,x_k)$ and
$xr=(x_1,\dots,x_k)(r_1,\dots,r_k)$ for $r \in R$. Observe that, although
formally $\Zm{m}$ is not contained in $R$, it makes sense to speak
of multiplication of elements from $R$ and $\Zm{m}$ ($(R,+)$ is
a $\Zm{m}$-module and we can easily define the corresponding scalar
multiplication in \fp). %as for example for $x, y\in \Zm{m}$ we have 
%\[ x g_i \cdot y g_j =
%\underbrace{(g_i + \cdots + g_i)}\limits_{x\text{-times}}
%\cdot \underbrace{(g_j + \cdots + g_j)}\limits_{y\text{-times}} =
%\underbrace{(g_ig_j + \cdots + g_ig_j)}\limits_{xy\text{-times}} = (xy)
%\cdot (g_ig_j).\]
The remaining steps follow as in the proof
of Theorem~\ref{theorem_reduction-ordings-lcon}.

\end{proof}
