# Supplementary material for: Definability of linear equation systems over groups and rings
Source: arXiv:1204.3022 source file (2013-11-11)
Supplement: Supplementary file 3 [file reductions-to-solvability.tex]

\setcounter{theorem}{12}

\lemmanormalformles*

\begin{proof}
We describe the interpretation $\mathcal I$ as the composition of
three quantifier-free transformations of linear equation systems. The
first transformation maps a system $(A, \fvec b)$ over $R$ to an
equivalent system $(B, \fvec c)$ over the ring $\Zm m$, where $m$ is
the characteristic of $R$. Secondly, $(B, \fvec c)$ is mapped to an
equivalent system $(C, \fvec 1)$ over $\Zm m$; i.e. to a system where
the right-hand side of each equation is the constant 1. Finally, we
transform $(C, \fvec 1)$ into an equivalent system $(D, \fvec 1)$ over
$\Zm m$, where $D$ is a $\{0,1\}$-matrix.

The first transformation is obtained by the adapting the proof of
Theorem~\ref{theorem_reduction-ordings-lcon}, which gave a fixed-point
reduction from the solvability problem over ordered rings to
solvability over cyclic groups. More specifically, the reduction maps
a linear equation system over an ordered ring $R$ to an equivalent
system over the characteristic subring of $R$, seen as a cyclic group.
Reviewing the proof, it can be seen that first-order quantifiers and
fixed-point operators are only needed for the decomposition of the
ring $R$ into its local summands and, for each local summand, for the
decomposition into a direct sum of cyclic groups. It follows that when
the underlying ring is fixed, as in our case, these decompositions can
be defined by fixed quantifier-free formulae. Hence, there is a
quantifier-free transformation of the system $(A, \fvec b)$ over the
fixed ring $R$ to an equivalent system $(B, \fvec c)$ over the fixed
ring $\Zm m$.

For the second transformation, suppose that $B$ is an $I \times J$
matrix and $\fvec c$ a vector indexed by $I$. We define a new linear
equation system $\struct T$ over $\Zm m$ in which the right-hand side
of every equation is the constant 1. The system $\struct T$ has, in
addition to all the variables that occur in $\struct S$, a new
variable $v_e$ for every $e \in I$ and a new variable $w_r$ for every
$r \in R$. For every element $r \in \Zm m$, we include in $\struct T$
the equation $(1-r)w_1 + w_r= 1$. It can be seen that this subsysem of
equations has a unique solution given by $w_r = r$ for all $r \in \Zm
m$. Finally, for every equation $\sum_{j \in J} B(e,j) \cdot x_j =
\fvec c(e)$ in $\struct S$ (indexed by $e \in I$) we include in
$\struct T$ the two equations $v_e + \sum_{j \in J} B(e,j) \cdot x_j =
1$ and $v_e + w_{\fvec c(e)}= 1$. By solving the latter equation for
$v_e$ and inserting the result into the former equation, it can be
seen that the system $\struct T$ is equivalent to $\struct S$ and can
be written as $C \cdot \fvec x = \fvec 1$, where $C$ is a matrix over
$\Zm m$. 

Finally, we translate the linear equation system $\struct T: C \fvec x
= \fvec 1$ over $\Zm m$ to an equivalent system over $\Zm m$ in which
all scalar coefficients and constant values are either 0 or 1. As a
first step, we translate $\struct T$ to an intermediate system
$\struct U'$, defined as follows. For each variable $v$ in $\struct
T$, the system $\struct U'$ has the $m$ distinct variables $v_0,
\dots, v_{m-1}$ together with equations $v_i = v_j$ for $i\not= j$. We
also include in $\struct U'$ the equation obtained by replacing, in
each equation of $\struct T$, each term of the kind $rv$ by the term
$\sum_{1 \leq i \leq r} v_i$. Since for each $v$, the variables $v_i$
all have to take the same value, it follows that $\struct U'$ is
equivalent to $\struct T$. However, in order to establish our original
claim we need to rewrite the auxiliary equations of the form $v_i =
v_j$ as a set of equations whose right-hand sides are equal to 1. To
achieve this, we introduce a new variable $v_j^-$ for each $v_j$,
together with the equation $v_j + v_j^- + v_1 = 1$. Finally, we
rewrite each equation $v_i = v_j$ as $v_i + v_j^- + v_1 = 1$. It can
be seen that the resulting system $\struct U$ is equivalent to
$\struct U'$ and has the form $D \cdot \fvec x = \fvec 1$, where $D$
is a $\{0,1\}$-matrix. 
\begin{detailedproof}
\medskip

\noindent
Since the ring $R$, and hence also the ring $\Zm m$, is fixed, it can
be seen that all the reductions we have outlined above can be
formalised as quantifier-free reductions, which proves our claim.
\end{detailedproof}
\end{proof}

\setcounter{theorem}{14}

\lemmahermitenormalform*

\begin{proof}
 If $R$ is not a field, fix an element $\pi \in R$ such that the
maximal ideal in $R$ is $m = \pi R$. Then, every element of $R$ can be
represented in the form $\pi^n u$ where $n\geq 0$ and $u \in U(R)$. It
follows that for all elements $r, s \in R$ we have $r \divides s$ or
$s \divides r$. Now, consider the following procedure: In the
remaining $k \times \ell$-matrix, choose an entry $r \in R$ which is
minimal with respect to divisibility and use row and column
permutations to obtain an equivalent $k \times \ell$-matrix $A^\prime$
which has $r$ in the upper left corner, i.e.\ $A^\prime(1,1) = r$.
Then, use the first row to eliminate all other entries in the first
column. After this transformation, the element $r$ still divides every
entry in the resulting matrix, since all of its entries are linear
combinations of entries of $A^\prime$. Proceed with the $(k-1) \times
(\ell -1)$-submatrix which results by deleting the first row and
column
from $A^\prime$.
\end{proof}

\setcounter{theorem}{21}

\begin{lemma}
\label{lemma_appendix-redtosolv-nonppm}
 Let $\mathcal{I}$ be a first-order interpretation of $\vocLinEqRingFixed{\Zm{m}}$ in a signature $\tau$, where $m = p_1^{n_1} \cdots p_k^{n_k}$ for pairwise distinct primes $p_1, \dots, p_k$ and natural numbers $n_1, \dots, n_k \geq 1$. Then there exists a first-order interpretation $\mathcal{J}$ of $\vocLinEqRingFixed{\Zm{m}}$ such that $\qr(\mathcal I) = \qr(\mathcal J)$ and for all $\tau$-structures $\struct{A}$ we have $\mathcal{I}(\struct{A}) \not\in \clsles{R}$ if, and only if, $\mathcal{J}(\struct{A}) \in \clsles{R}$.
\end{lemma}
\begin{proof}
Let $(A, \fvec b)$ be a linear equation system over $\Zm{m}$ with coefficient matrix $A$ and solution vector $\fvec b$. We explain how to transform $(A,\fvec b)$ into a linear equation system $(A^\prime, \fvec b^\prime)$ over $\Zm{m}$, such that $(A, \fvec b)$ is not solvable if, and only if, $(A^\prime, \fvec b^\prime)$ is solvable. From the construction it will become clear that all necessary transformations can be defined from $\mathcal{I}$ without increasing the quantifier-rank of the respective formulas.

First, we use the Chinese remainder theorem and obtain a sequence of linear equations systems $(A_1, \fvec b_1), \dots, (A_k, \fvec b_k)$ over the local rings $\Zm{p_1^{n_1}}, \dots,  \Zm{p_k^{n_k}}$ such that the linear equation system $(A,\fvec b)$ is not solvable if, and only if, for some $1\leq i \leq k$ the linear system $(A_i, \fvec b_i)$ is not solvable. At this point, we apply Lemma \ref{lemma_criterion_non_solvability} to the systems $(A_i, \fvec b_i)$ and obtain new linear equation systems $(A_i^\prime, \fvec b_i^\prime)$ over $\Zm{p_i^{n_i}}$ which are solvable if, and only if, the linear systems $(A_i, \fvec b_i)$ are not solvable. We apply Lemma \ref{lemmanormalformles} to guarantee that all linear systems $(A_i^\prime, \fvec b_i^\prime)$ over $\Zm{p_i^{n_i}}$ are defined with solution vector $\fvec{1}$. 

In order to construct $(A^\prime, \fvec b^\prime)$, it remains to formalize the logical disjunction over  solvability of the linear systems $(A_i^\prime, \fvec b_i^\prime)$ by means of a linear equation system. To this end, we first combine all linear equation systems $(A_i^\prime, \fvec b_i^\prime)$ as independent subsystems in $(A^\prime, \fvec b^\prime)$. For this embedding we use the isomorphisms $(m/p_1^{n_1}\cdots p_{i-1}^{n_{i-1}} p_{i+1}^{n_{i+1}} \cdots p_k^{n_k}) \Zm{m} \simeq \Zm{p_i^{n_i}}$ and (independently) apply Lemma \ref{lemmanormalformles} again to maintain for all  subsystems $(A_i^\prime, \fvec b_i^\prime)$ the solution vector $\fvec{1}$. Now, again independently for each of the linear subsystems  $(A_i^\prime, \fvec b_i^\prime)$, we do the following: We extend each equation by three new variables $x^i$ and $y^i$ and $z^i$ (all with coefficient $1$) and introduce new equations $x^i=(p_1^{n_1-1}\cdots p_k^{n_k-1})$ and  $(p_1^{n_1-1}\cdots p_k^{n_k-1}) y^i = (p_1^{n_1-1}\cdots p_k^{n_k-1})$. These equations guarantee that (in a solution) $y^i = 1 + r(p_1p_2\cdots p_k)$ for some $r \in \Zm{m}$, hence the value of $y^i$ is a unit. Substituting the solution vectors $\fvec{1}$ by the vector containing the entry $p_1^{n_1-1}p_2^{n_2-1} \cdots p_k^{n_k-1}$ only, we thus obtain equivalent linear subsystems~$(A_i^\prime, \fvec b_i^\prime)$. At this point, we remove again all variables $x^i$ from the equations in the subsystem $(A_i^\prime, \fvec b_i^\prime)$ which leaves us with trivially solvable subsystems $(A_i^\prime, \fvec b_i^\prime)$.

Finally, the variables $z^i$ come into play: We extend the system $(A^\prime, \fvec b^\prime)$ by the equation $\sum_i z^i = p_1^{n_1-1} \cdots p_k^{n_k-1}$. This equation guarantees that (in a solution), there is at least one $1 \leq i \leq k$ such that $z^i \not= 0$. We make the following observation: Every element $r \in \Zm{m}$ divides $p_1^{n_1-1} \cdots p_k^{n_k-1}$. For units, this is clear, so let $r \in \Zm{m}$ be a non-unit. Then we can express $r$ as $r=p_1^{l_1} \cdots p_k^{l_k} s$, where $l_1, \dots, l_k \geq 0$, $s$ is co-prime to $m$ and for at least one $1 \leq i \leq k$ we have $l_i \geq 1$. However, since $s$ is a unit in $\Zm{m}$, the claim follows. With this observation it is immediate, that the linear subsystem $(A_i^\prime, \fvec b_i^\prime)$ for which $z^i \not= 0$ has to be solvable. Moreover it is clear, that in the case where $(A_i^\prime, \fvec b_i^\prime)$ is solvable, we can set $z^i = p_1^{n_1-1} \cdots p_k^{n_k-1}$ and $z^j = 0$ for all $j \not=i$ in a solution for $(A_i^\prime, \fvec b_i^\prime)$. 
\end{proof}
