# Supplementary material for: Definability of linear equation systems over groups and rings
Source: arXiv:1204.3022 source file (2013-11-11)
Supplement: Supplementary file 5 [file linear-algebra-fpc-proofs.tex]

%--- Size of the general linear group -----------------------------------------
\begin{lemma}
\label{lemma_cardinality-gen-lin-group}
Let $R$ be a finite local ring with maximal ideal $m$ and let $I$  be a finite set of size $n > 0$. If we denote the residue field $R / m$ by $k$ and its cardinality by $q \defeq \card{k}$ then we have
\[ 
	\card{\genl{I}{k}} = q^{n^2} \cdot \prod_{i=0}^{n-1} (1-q^{i-n}) 
	\quad\text{ and }\quad
	\card{\genl{I}{R}} = \card{R}^{n^2} \cdot \prod_{i=0}^{n-1} (1-q^{i-n}).
\]
\end{lemma}

\begin{proof} 
The first equation is common knowledge: An $I \times I$ matrix over $k$ is invertible if and only if its columns are linearly independent. Each set of $i$ linearly independent columns gives rise to $q^i$ different linear combinations. Thus, there remain $(q^{n}  - q^i)$ many linearly independent columns. This counting argument shows that
\begin{align*}
	\card{\genl{I}{k}} &= (q^{n} -1 ) \cdot (q^{n} - q ) \cdot (q^{n} -q^2 ) \cdots (q^{n} -q^{n-1} ) =  \prod_{i=0}^{n-1} (q^{n} - q^i ).
\end{align*}

\noindent
To derive the second equation, consider the canonical group homomorphism $\pi: \genl{I}{R} \ra \genl{I}{k}$. It is easy to see that $\card{\mathrm{ker}(\pi)} = \card{m}^{n^2}$. The fundamental homomorphism theorem thus implies that $\card{\genl{I}{\struct R}} =  {\card{m}^{n^2}} \card{\genl{I}{k}}$ which proves the second identity since $q \cdot \card{m} = \card{R}$.
\end{proof}

%--- Size of the general linear group -----------------------------------------
\lemmaCardinalityGenLin*

\begin{proof} 
By Lemma~\ref{lemma_cardinality-gen-lin-group}, we have an exact expression for the cardinality of $\card{\genl{I}{R}}$ for any non-empty set $I$ and any finite local ring $R$. It is straightforward to verify that the binary encoding of this expression can be formalised by a formula and a number term of fixed-point logic with counting.
\end{proof}
